# Supplementary material for: Fill-Up: Balancing Long-Tailed Data with Generative Models
Source: arXiv:2306.07200 source file (2023-06-12)
Supplement: Supplementary file 1 [file CLIP_templete.tex]

\begin{table}[]
\centering
\resizebox{0.92\textwidth}{!}{
\begin{tabular}{lccccccccl}
\cmidrule[1.0pt]{1-10}
\multicolumn{10}{c}{\textbf{CLIP templetes}}  \\
\cmidrule[1.0pt]{1-10}
a bad photo of a \{\texttt{CLS}\} & &&&&&&&& a cropped photo of a \{\texttt{CLS}\}.\\
a photo of many \{\texttt{CLS}\}. & &&&&&&&& a plastic \{\texttt{CLS}\}.\\
a sculpture of a \{\texttt{CLS}\}. & &&&&&&&& a plastic \{\texttt{CLS}\}.\\
a photo of the hard to see \{\texttt{CLS}\}. & &&&&&&&& a plastic \{\texttt{CLS}\}.\\
a low resolution photo of the \{\texttt{CLS}\}. & &&&&&&&& a plastic \{\texttt{CLS}\}.\\
graffiti of a \{\texttt{CLS}\}. & &&&&&&&& a plastic \{\texttt{CLS}\}.\\
a bad photo of the \{\texttt{CLS}\}. & &&&&&&&& a plastic \{\texttt{CLS}\}.\\
a cropped photo of the \{\texttt{CLS}\}. & &&&&&&&& a plastic \{\texttt{CLS}\}.\\
a tattoo of a \{\texttt{CLS}\}. & &&&&&&&& a plastic \{\texttt{CLS}\}.\\
the embroidered \{\texttt{CLS}\}. & &&&&&&&& a plastic \{\texttt{CLS}\}.\\
a photo of a hard to see \{\texttt{CLS}\}. & &&&&&&&& a plastic \{\texttt{CLS}\}.\\
a bright photo of a \{\texttt{CLS}\}. & &&&&&&&& a plastic \{\texttt{CLS}\}.\\
a photo of a clean \{\texttt{CLS}\}. & &&&&&&&& a plastic \{\texttt{CLS}\}.\\
a photo of a dirty \{\texttt{CLS}\}. & &&&&&&&& a plastic \{\texttt{CLS}\}.\\
a photo of many \{\texttt{CLS}\}. & &&&&&&&& a plastic \{\texttt{CLS}\}.\\
a photo of many \{\texttt{CLS}\}. & &&&&&&&& a plastic \{\texttt{CLS}\}.\\
a photo of many \{\texttt{CLS}\}. & &&&&&&&& a plastic \{\texttt{CLS}\}.\\
a photo of many \{\texttt{CLS}\}. & &&&&&&&& a plastic \{\texttt{CLS}\}.\\
a photo of many \{\texttt{CLS}\}. & &&&&&&&& a plastic \{\texttt{CLS}\}.\\
a photo of many \{\texttt{CLS}\}. & &&&&&&&& a plastic \{\texttt{CLS}\}.\\
a photo of many \{\texttt{CLS}\}. & &&&&&&&& a plastic \{\texttt{CLS}\}.\\
a photo of many \{\texttt{CLS}\}. & &&&&&&&& a plastic \{\texttt{CLS}\}.\\
a photo of many \{\texttt{CLS}\}. & &&&&&&&& a plastic \{\texttt{CLS}\}.\\
\cmidrule[1.0pt]{1-10}
\end{tabular}}
\end{table}
