# Supplementary material for: Fill-Up: Balancing Long-Tailed Data with Generative Models
Source: arXiv:2306.07200 source file (2023-06-12)
Supplement: Supplementary file 2 [file 5_ensemble.tex]

\section{Ensembling methods}
\label{sup_ensembling}
